# Supplementary material for: Intensity interferometry for ultralight bosonic dark matter detection
Source: arXiv:2202.02645 source file (2023-05-17)
Supplement: Supplementary file 1 [file EliminatedAppendix.tex]

\DKIns{To see how the expression \eqref{eq:g0approx} is related to the sensitivity of a search for a UBDM signal, consider the case of atomic magnetometers used to detect the pseudo-magnetic field described by Eq.~\eqref{eq:pseudo-magnetic-field}. 
For simplicity, let us assume the sensitive axes of the magnetometers are oriented in the same direction (see Sec.~\ref{app:AngleDep}) and are otherwise identical. 
Based on Eq.~\eqref{eq:ALP-intensity-gradient}, the UBDM signal obtained from the cross-correlation measurement, averaged over many coherence times ($T \gg \tau_c$), is given by
\begin{align}
    \kappa_A \kappa_B \langle s^2 (\tau) \rangle_t \approx \prn{ \frac{\hbar^3 \rho\ts{dm} v_0}{g_F \mu_B m_\varphi f_q^2} }^2 \mc{F}(\tau)~,
\end{align}
where $\mc{F}(\tau)$ is a lineshape function describing the $\tau$-dependence of $g^{(1)}_{AB}(\tau)$ as shown in Fig.~\ref{fig:g1}. 
Based on Eq.~\eqref{eq:min-field}, the product of the average uncorrelated noise in the two identical magnetometers is described by 
\begin{align}
    \sigma_A \sigma_B \approx \frac{\prn{\delta B}^2}{\Delta\tau}~,
\end{align}
where $\Delta \tau$ is the step size of time (or bin size) of the measured cross-correlation data (recall that $\delta B$ is in units of, for example, ${\rm pT/\sqrt{Hz}}$, and $\sigma_A\sigma_B$ is in units of ${\rm pT^2}$).
Thus in the presence of a nonzero UBDM signal the measured cross-correlation would be}
\begin{equation}
	g^{(1)}_{AB}(\tau)\ts{sig} \approx \prn{ \frac{\hbar^3 \rho\ts{dm} v_0}{g_F \mu_B \delta B m_\varphi f_q^2} }^2 \mc{F}(\tau) \Delta \tau ~.
	\label{eq:gTauSig}
\end{equation}

\DKIns{In the absence of a UBDM signal, the cross-correlation measurement is dominated by the noise term, which can be estimated as a random walk of average step size $(\delta B)^2/\Delta \tau$ with $T/\Delta \tau$ steps, averaged over time $T$,}
\begin{align}
    \langle \mc{N}_A(t) \mc{N}_B (t+\tau) \rangle_t \approx \frac{\prn{\delta B}^2}{\sqrt{ T \Delta\tau }}~,
\end{align}
so that
\begin{equation}
	g^{(1)}_{AB}(\tau)\ts{noise} \approx \sqrt{\frac{\Delta \tau}{T}}~.
	\label{eq:gTauNoise}
\end{equation}
Thus we find for the signal-to-noise for a given value of $\tau$ is given by:
\begin{align}
    \prn{\rm{S/N}}\ts{pair} (\tau) & = \frac{g^{(1)}_{AB}(\tau)\ts{sig}}{g^{(1)}_{AB}(\tau)\ts{noise}} ~, \\
    &\sim  \prn{ \frac{\hbar^3 \rho\ts{dm} v_0}{g_F \mu_B \delta B m_\varphi f_q^2} }^2 \mc{F}(\tau) \sqrt{ T \Delta\tau }~.
    \label{eq:StoN1pt}
\end{align}

\DKIns{The amplitude of the UBDM signal can be extracted, for example, by fitting the measured $g^{(1)}_{AB}(\tau)$ to $\mc{F}(\tau)$, and Eq.~\eqref{eq:gTauNoise} estimates the point-to-point fluctuations of the fit residuals that determine the uncertainty in the measured amplitude. Therefore, taking into account the $\sim (T/\Delta\tau)$ values of $g^{(1)}(\tau)$ from $0 \lesssim \tau \lesssim T$, we obtain a signal-to-noise ratio $\prn{\rm{S/N}}$ integrated over all values of $\tau$
\begin{align}
    \prn{\rm{S/N}}\ts{pair} \sim T \prn{ \frac{\hbar^3 \rho\ts{dm} v_0}{g_F \mu_B \delta B m_\varphi f_q^2} }^2~.
\end{align}
For $N_m$ identical magnetometers, the number of pairs scales as $N_m(N_m-1)/2 \approx N_m^2/2$. Assuming the measurements in different pairs are Gaussian distributed about the mean, we obtain the scaling of the overall network signal-to-noise
\begin{align}
    \prn{\rm{S/N}}\ts{network} \sim N_m T \prn{ \frac{\hbar^3 \rho\ts{dm} v_0}{g_F \mu_B \delta B m_\varphi f_q^2} }^2~.
\end{align}
Setting $\prn{\rm{S/N}}\ts{network} \sim 1$ gives the sensitivity estimate described by Eq.~\eqref{eq:f_q-sens-mags}.}

\section{Signal-to-noise scaling with time and number of sensors}\label{app:SNscalingNate}
%%%%%%%%%%%%%%%%%%%%%%%%%%%%%%%%%%%%%%%%%%%%%%%%%%%%%%%%%%%%%%%%%%%%%%%%%%%%%%%%%%%
%%%%%%%%%%%%%%%%%%%%%%%%%%%%%%%%%%%%%%%%%%%%%%%%%%%%%%%%%%%%%%%%%%%%%%%%%%%%%%%%%%%

In the main text, we estimate the sensitivity of intensity interferometry with sensor networks to UBDM: see Figs.~\ref{Fig:sensitivity-GNOME} and \ref{Fig:sensitivity-clocks}, Eqs.~\eqref{eq:min-field}, \eqref{eq:f_q-sens-mags}, \eqref{eq:frac-freq-variation-clock-sens}, and surrounding text. Our sensitivity estimate assumes that the signal-to-noise ratio for an intensity-interferometry-based UBDM search will improve as $(NT)^{1/2}$, where $N$ is the number of sensors and $T$ is the measurement time. The reasons for this scaling with $N$ and $T$ are somewhat subtle; for example, in some other UBDM searches that measure for times much longer than the UBDM coherence time, the signal-to-noise ratio scales as $T^{1/4}$ \cite{Asz01,Asz10,budker2014proposal,Sik14,chaudhuri2015radio,phipps2020exclusion,manley2020searching,crescini2020axion,braine2020extended,backes2021quantum,Ayb21CASPErE,gramolin2021search} (a result of the fact that both the signal and the noise are stochastic). In this appendix we estimate the scaling of a prototypical analysis procedure in order to justify this $(NT)^{1/2}$ signal-to-noise scaling.

Let us consider two sensors (denoted by $A,B$) that output signals like the ones introduced in Appendix~\ref{app:search}: $\mc{S}_{A,B}(t) = \kappa_{A,B} s(t) + \mc{N}_{A,B}(t)$, and we will use $\kappa_{A,B} = 1$ for simplicity. Let us now examine two discrete time series of $\mc{S}_{A,B}(t)$ with $M$ points each: $x_A(t)$ and $x_B(t)$. These time series are taken from sensors $A$ and $B$ respectively and correspond to $\mc{S}_{A,B}$ sampled at the same times, ${t = [t_1,...,t_M]}$. Element-wise multiplication of both time series can be written as,
\begin{align}
    x_A x_B &= (s + \mc{N}_A)( s + \mc{N}_B) \\&= \mc{N}_A \mc{N}_B + (\mc{N}_A + \mc{N}_B)s + s^2,
\end{align}
for each of the elements; where the time dependence was omitted to simplify notation.

The noise in the sensors is assumed to be a Gaussian centered at zero, and with a variance of $\sigma^2$, i.e., $\mc{N} \sim \mc{G}(0,\sigma^2)$, while the expectation value of $s$ is zero (recall that the mean of $\mathcal{S}$ is zero by construction since the mean of the raw data is subtracted in the data preprocessing in order to calculate the cross-correlation). Then it follows that the expectation value for the individual elements of the multiplied time series $x_A x_B$ is
\begin{align}
    \EE[x_A x_B] &= \EE[s^2],
\end{align}
since for the cross terms $\EE[\mathcal{N}_A \mathcal{N}_B] = \EE[(\mathcal{N}_A + \mathcal{N}_B)s] = 0$.
The variance of the individual elements can be calculated using the identity
\begin{align}
    \VV[X] &= \EE[X^2] - (\EE[X])^2.
\end{align}
And for small signals (${\EE[\mc{N}^2] \gg \EE[s^2]}$), the variance ${\zeta^2 \equiv \VV[x_A x_B]}$ of the individual $x_A x_B$ elements will be approximately
\begin{align}
    \zeta^2 \approx  \EE[\mc{N}_A^2 \mc{N}_B^2]
\end{align}
(where we have assumed that $s$, $\mc{N}_A$, and $\mc{N}_B$ are independent, and therefore the expectation value of terms in $(x_A x_B)^2$ that are proportional to odd powers of $s$, $\mc{N}_A$, and $\mc{N}_B$ are 0). Let us now consider the average of the $M$ points of the multiplied time series,
\begin{align}
    \Gamma &\equiv \frac{1}{M} \sum^M_{i=1} x_A(t_i) x_B(t_i).
\end{align}
Note that this quantity is closely related to $g^{(1)}(0)$ (see Appendix~\ref{app:search}). Given a large enough $M$, we can use the central limit theorem, which states that $\Gamma$ will be approximately described by a Gaussian distribution with a mean and variance determined by those of their individual elements,
\begin{align}
    \Gamma &\sim \mathcal{G}(\EE[s^2], \zeta^2/M ) \label{eq:GaussianDMSensitive}.
\end{align}

By measuring several segments of $M$ points, one could obtain a measurement of $\Gamma$ with a determined uncertainty, i.e., $\Gamma = \overline{\Gamma} \pm \delta \Gamma$. Since we are interested in seeing how the signal-to-noise ratio of $s$ (and not $s^2$) scales, we can derive from the measured $\overline{\Gamma} \pm \delta \Gamma$ an estimate of $\overline{s} \pm \delta s$ using linear error propagation (which will be valid for a large enough $M$):
\begin{align}
    \overline{s} &= \sqrt{\overline{\Gamma}}\\
    \delta s &= \frac{\delta\Gamma}{2 \sqrt{\overline{\Gamma}}}.
\end{align}

From Eq.~\eqref{eq:GaussianDMSensitive} it follows that the uncertainty on $\Gamma$ is,
\begin{align}
    \delta \Gamma &\propto \sqrt{\frac{\zeta^2}{M}}.
\end{align}

Therefore, the signal to noise $\overline{s} / \delta s$ (ie. how many standard deviations is the mean away from zero) will be

\begin{align}
    \frac{\overline{s}}{\delta s} = \frac{2 \overline{\Gamma}}{\delta \Gamma} \propto M^{1/2}.
\end{align}

For a fixed number of segments of the data, it is clear that $M \propto T$; i.e., if one took twice the amount of data points ($T \rightarrow 2T$), then the individual segments would be twice as long ($M \rightarrow 2M$). The same argument applies to the number of sensors, since the number of independent measurements of $\Gamma$ would be proportional to the number of sensor pairs.
